# Supplementary material for: Enhancing gravitational-wave burst detection confidence in expanded detector networks with the BayesWave pipeline
Source: arXiv:2102.10816 source file (2021-02-22)
Supplement: Supplementary file 1 [file appendix3.tex]

\section{HL versus HLV Bayes Factors} \label{app:BF_shift}

\begin{figure}[t]
\centering
\includegraphics[width=.49\textwidth]{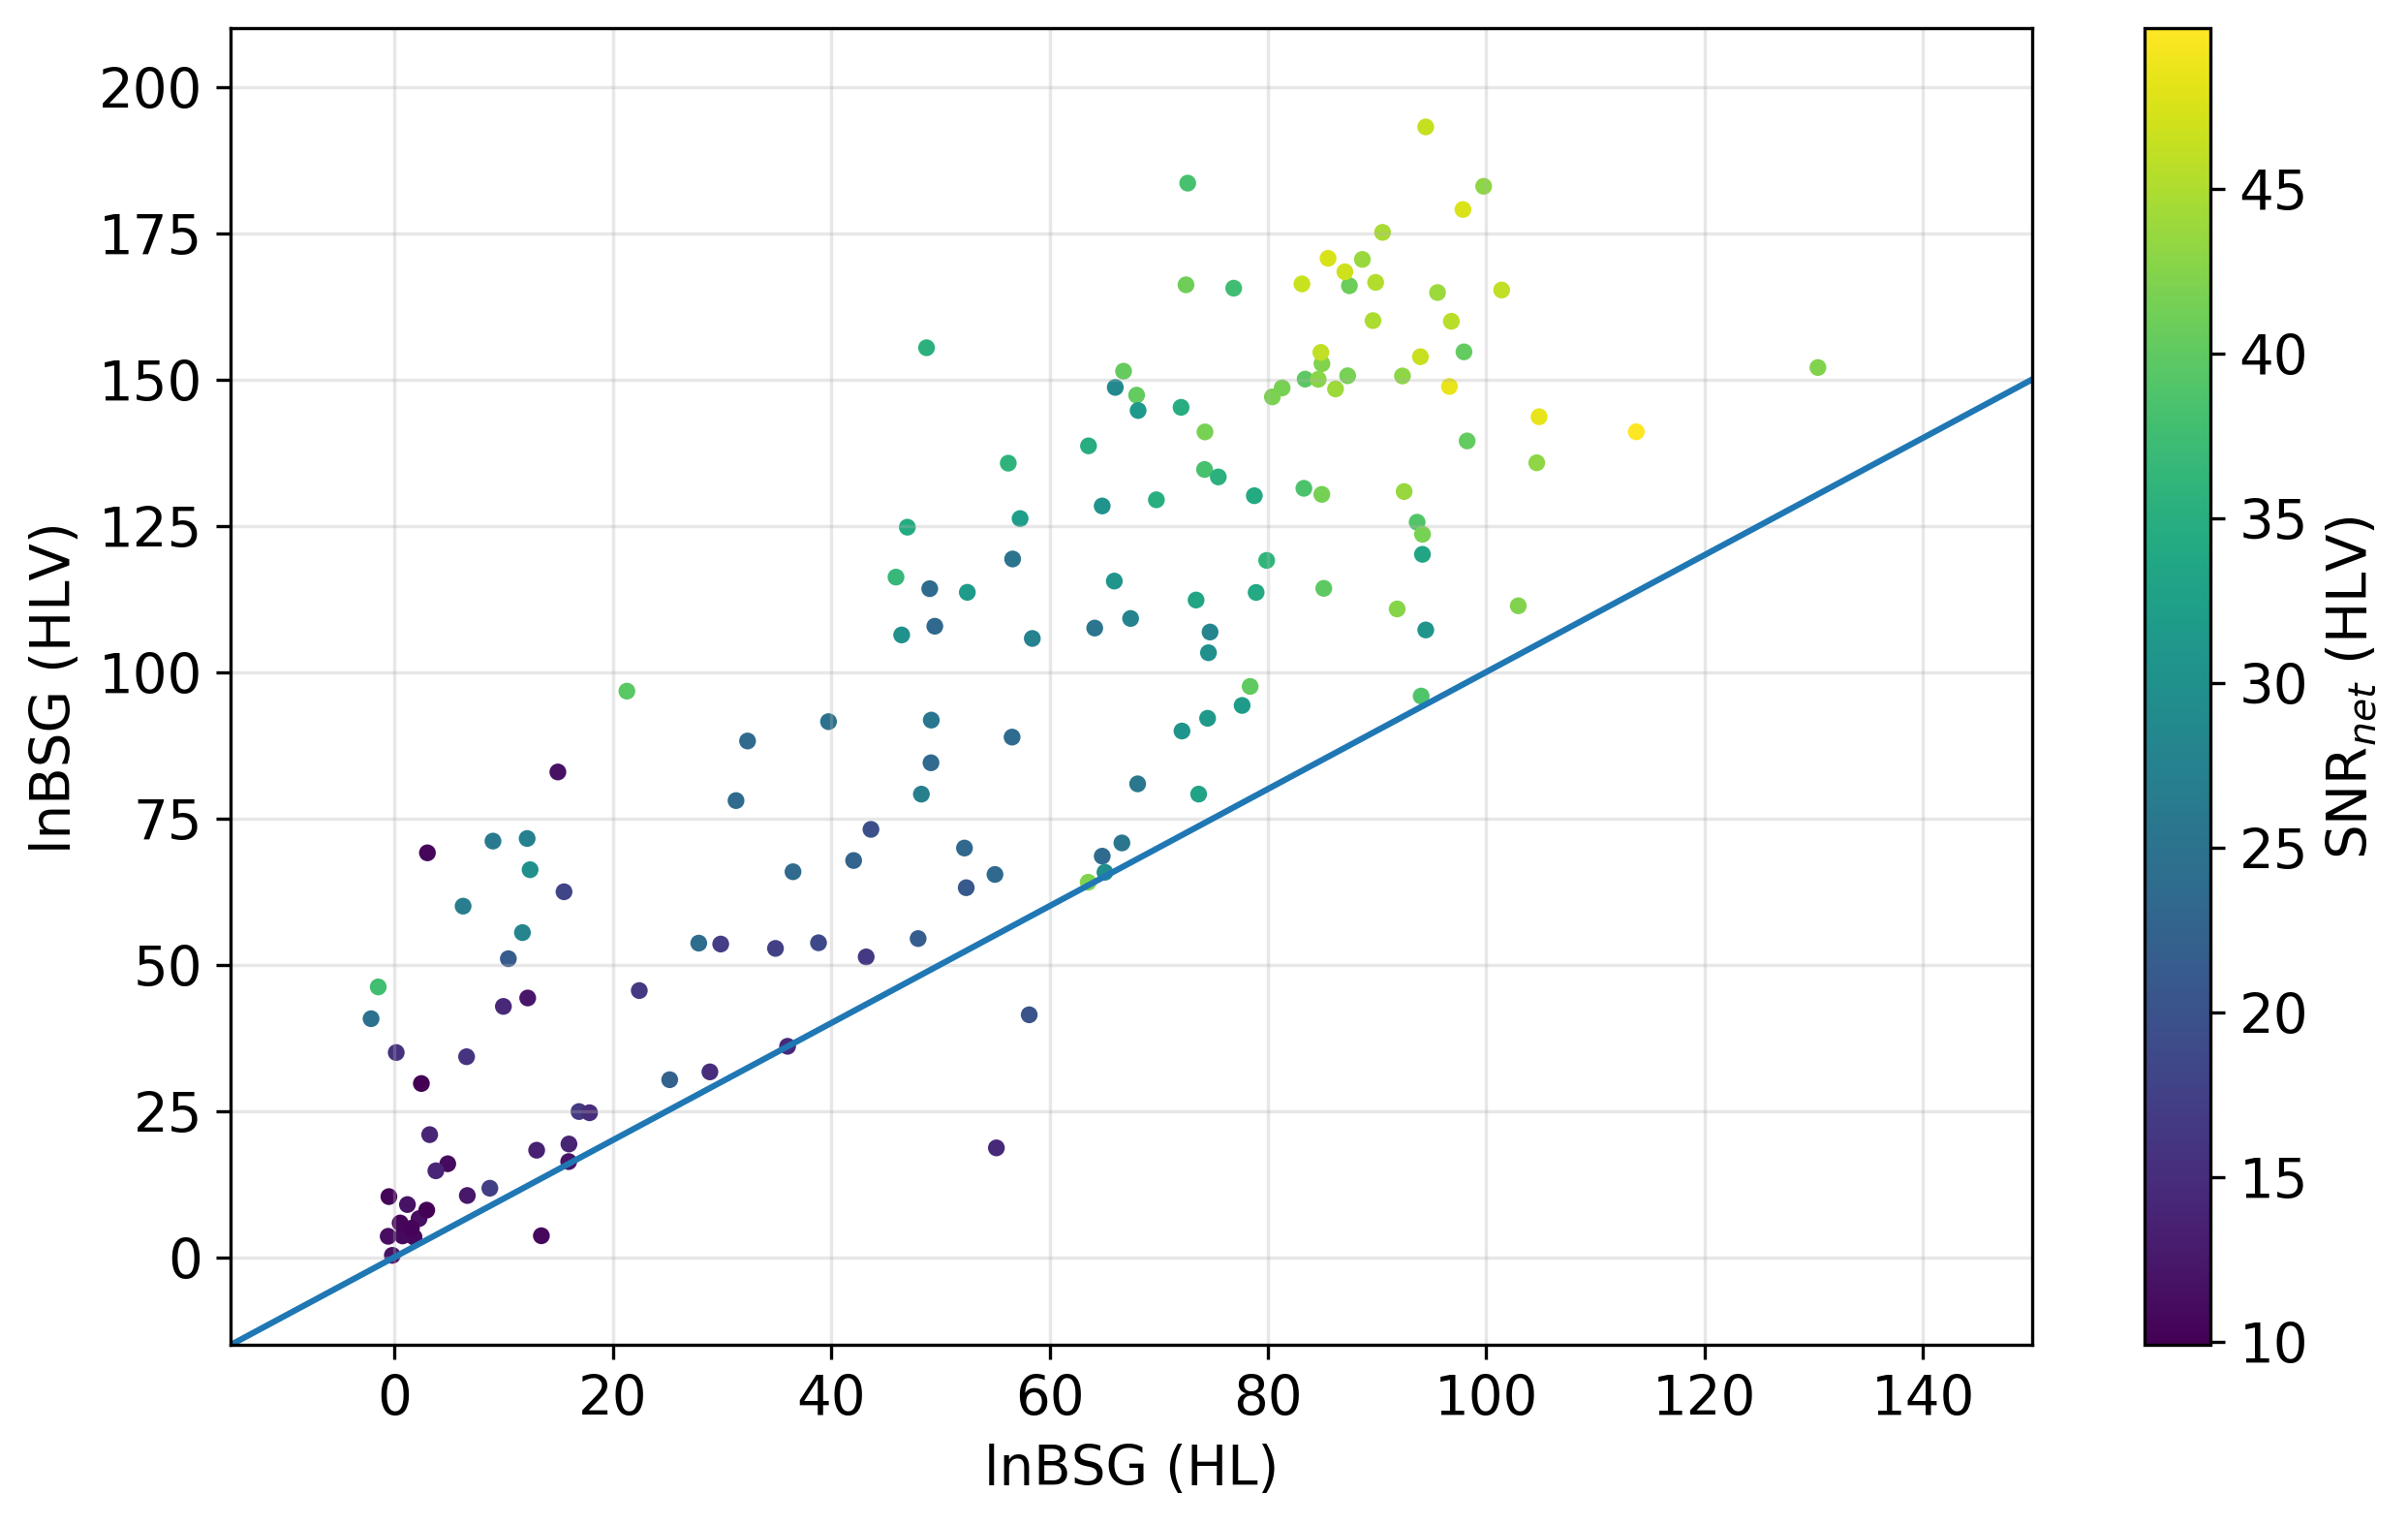}
    \caption{Log signal-to-glitch Bayes factor, $\ln \mathcal{B}_{\mathcal{S},\mathcal{G}}$ of the HLV network versus that of the HL network and the color bar shows the SNR$_\text{net}$ of the HLV network for each injection.}
    \label{fig:BF_HLVsnr}
\end{figure}

%In the top left panel of Figure \ref{fig:BSG} in Section \ref{sec:BayesFactor}, we show the relationship between $\ln \mathcal{B}_{\mathcal{S},\mathcal{G}}$ and the network SNRs of the respective detector. 
Since the waveforms injected into both detector networks (HL and HLV) are identical in Section \ref{sec:BayesFactor}, we can do a one-to-one comparison of the Bayes factors per injection. HLV network injections generally have higher SNR$_\text{net}$ compared to those in the HL network, so the $\ln \mathcal{B}_{\mathcal{S},\mathcal{G}}$ of the same injection between the two networks do not line-up at the same SNR$_\text{net}$ as seen in the top left panel of Figure \ref{fig:BSG}. This makes it difficult to compare them. 

%Another way of presenting the result in Figure \ref{fig:BSG} shown in the left panel of Figure \ref{fig:BF_HLVsnr}, which is to plot the HL network $\ln \mathcal{B}_{\mathcal{S},\mathcal{G}}$ against the HLV network SNR rather than the HL network SNR. By doing so, we shift the SNR of the injection in the HL network to match that of the HLV network so that a direct comparison can be made between $\ln \mathcal{B}_{\mathcal{S},\mathcal{G}}$ of the two networks for the same injection. Although the shifting of data points no longer gives the true relationship between $\ln \mathcal{B}_{\mathcal{S},\mathcal{G}}$ and SNR$_\text{net}$ for the HL network, having $\ln \mathcal{B}_{\mathcal{S},\mathcal{G}}$ of the HL and HLV network lining up at the same SNR$_\text{net}$ allows us to visually compare $\ln \mathcal{B}_{\mathcal{S},\mathcal{G}}$ for the same injected waveforms.
%The SNR of injection in the HL network is now shifted to align with data points of the same injection for the HLV network. 
%We can also shift $\ln\mathcal{B}_{\mathcal{S},\mathcal{G}}$ of the HLV network to line-up that of the HL network at the same SNR$_\text{net}$ to make the comparison.

In Figure \ref{fig:BF_HLVsnr} we show an explicit comparison between the $\mathcal{B}_{\mathcal{S},\mathcal{G}}$ of the HL and HLV networks. The line indicates equal $\ln\mathcal{B}_{\mathcal{S},\mathcal{G}}$ for both detector networks. Data points above the line are injections with higher $\mathcal{B}_{\mathcal{S},\mathcal{G}}$ in the HLV network compared to the HL network. The colours of the data points label the SNR of the injection in the HLV network. 
%Again, there is no specific reason why the HLV network SNR is indicated rather than the HL network SNR as they lead to the same interpretation. 
With a few exceptions, we can see from the right panel of Figure \ref{fig:BF_HLVsnr} that the recovered $\ln \mathcal{B}_{\mathcal{S},\mathcal{G}}$ for most injections is higher for the HLV network than the HL network at all SNR, although the difference in $\ln \mathcal{B}_{\mathcal{S},\mathcal{G}}$ between the two network becomes increasingly obvious at higher SNR. 

By Equation \ref{eq:BFscaleapprox}, the improvement in Bayes factor when adding a third detector to the network should be $50\%$. The best-fit least square, linear regression line for the data has a slope of 1.34 which indicates an average $34\%$ improvement in the Bayes factors with the addition of the Virgo detector. The analytic prediction is based on optimal scenarios, so although the empirical improvement in Bayes factor is slightly smaller than the analytic prediction, they still show reasonable agreement.
