# Supplementary material for: Enhancing gravitational-wave burst detection confidence in expanded detector networks with the BayesWave pipeline
Source: arXiv:2102.10816 source file (2021-02-22)
Supplement: Supplementary file 2 [file appendix4.tex]

\begin{figure*}[t]
\centering
\begin{minipage}{0.47\textwidth}
\includegraphics[width=\textwidth]{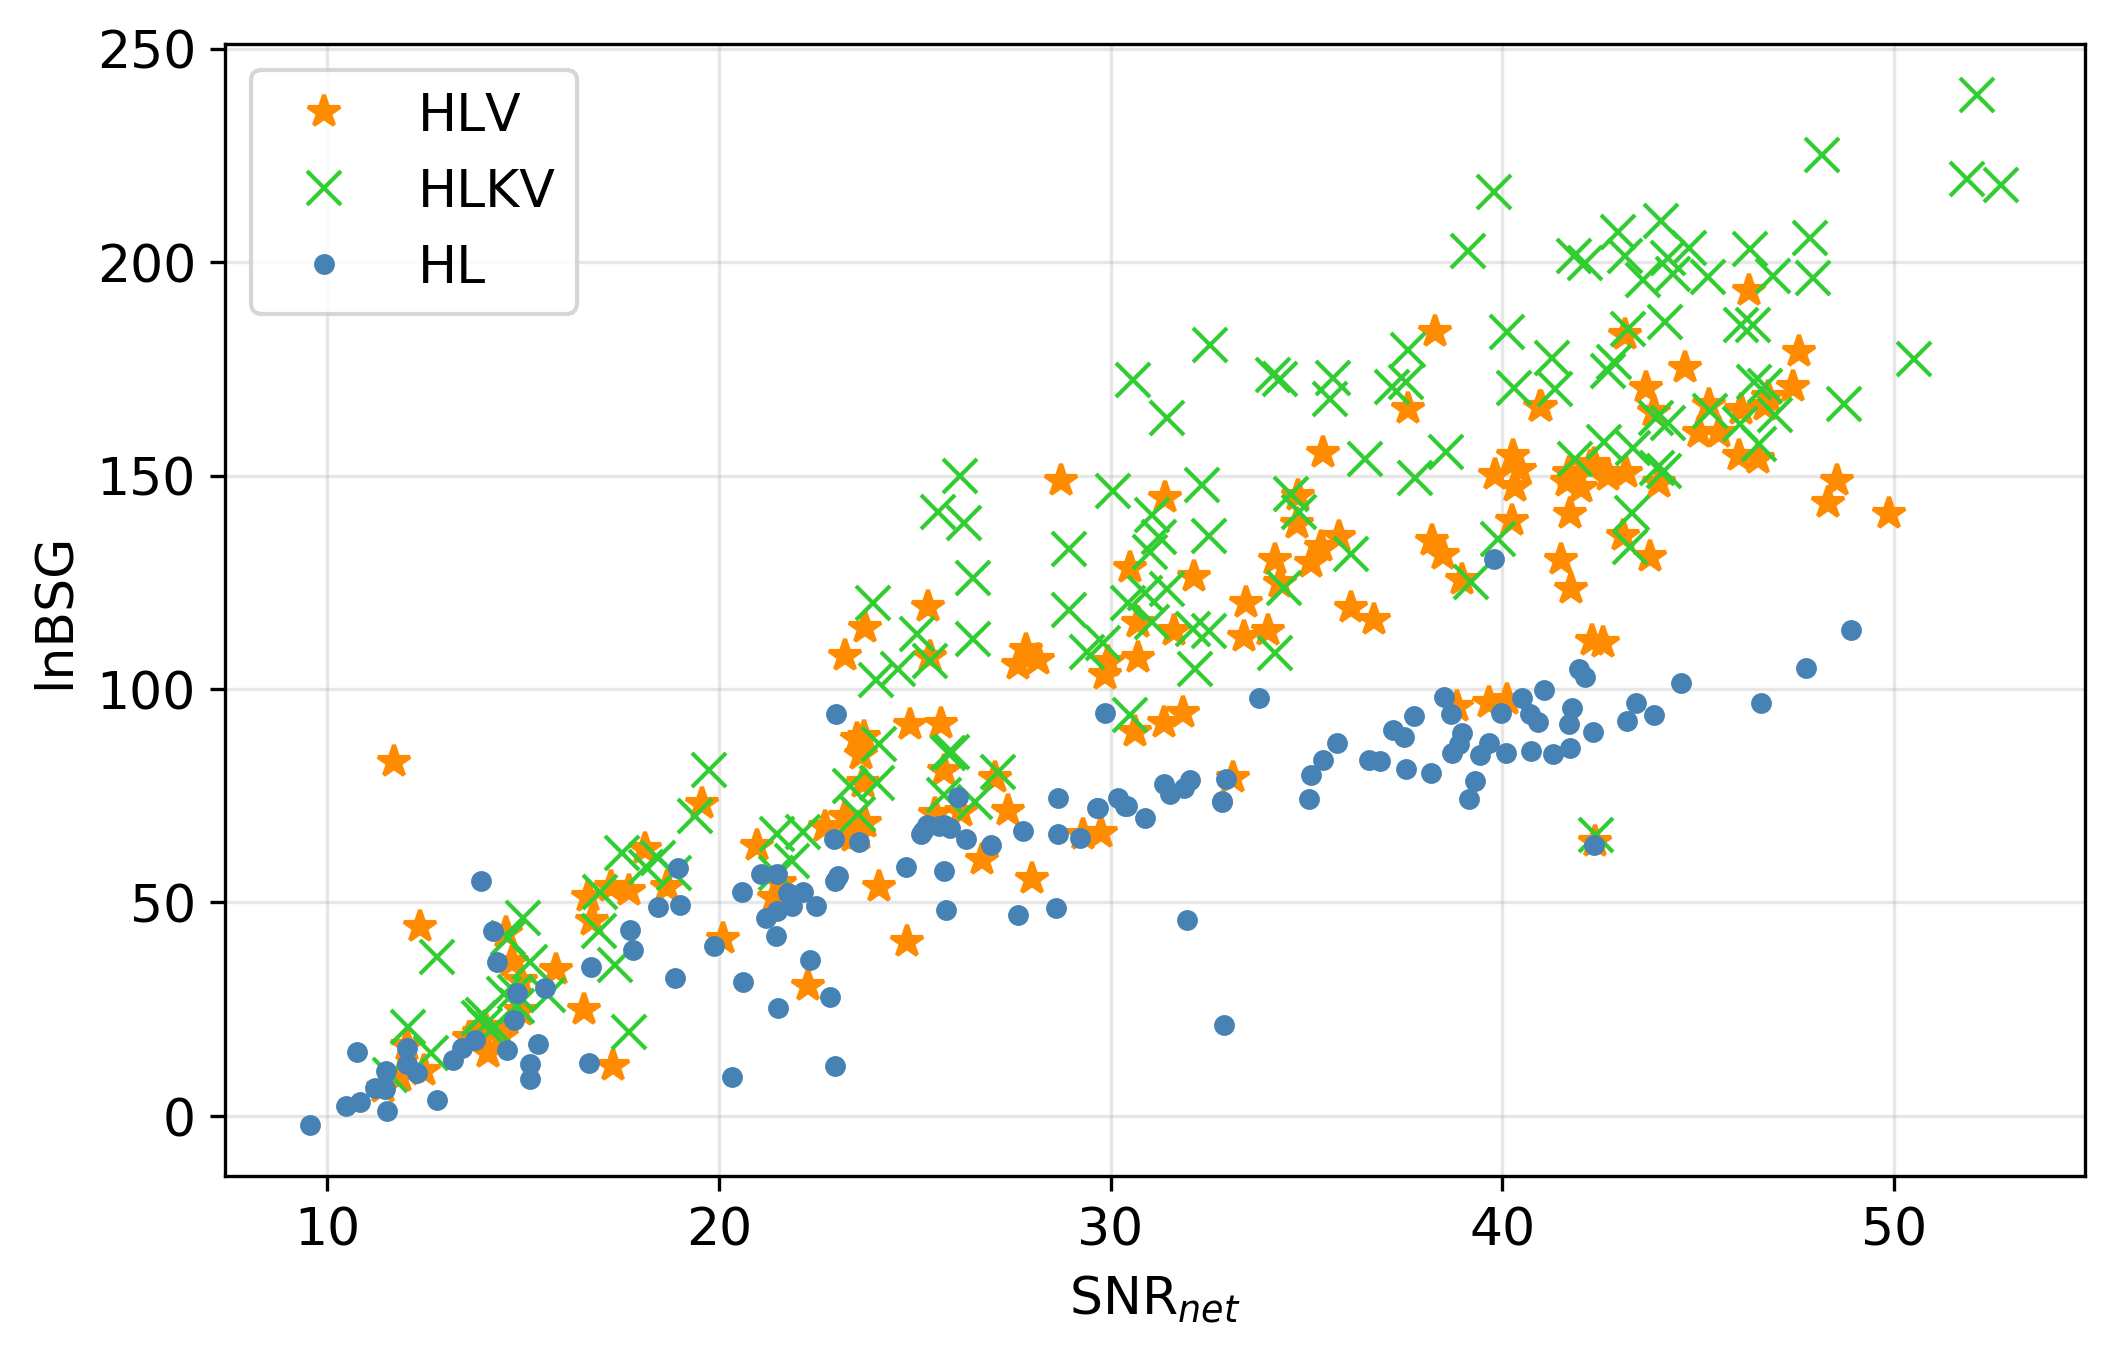}
\end{minipage}\hfill
\begin{minipage}{0.47\textwidth}
\includegraphics[width=\textwidth]{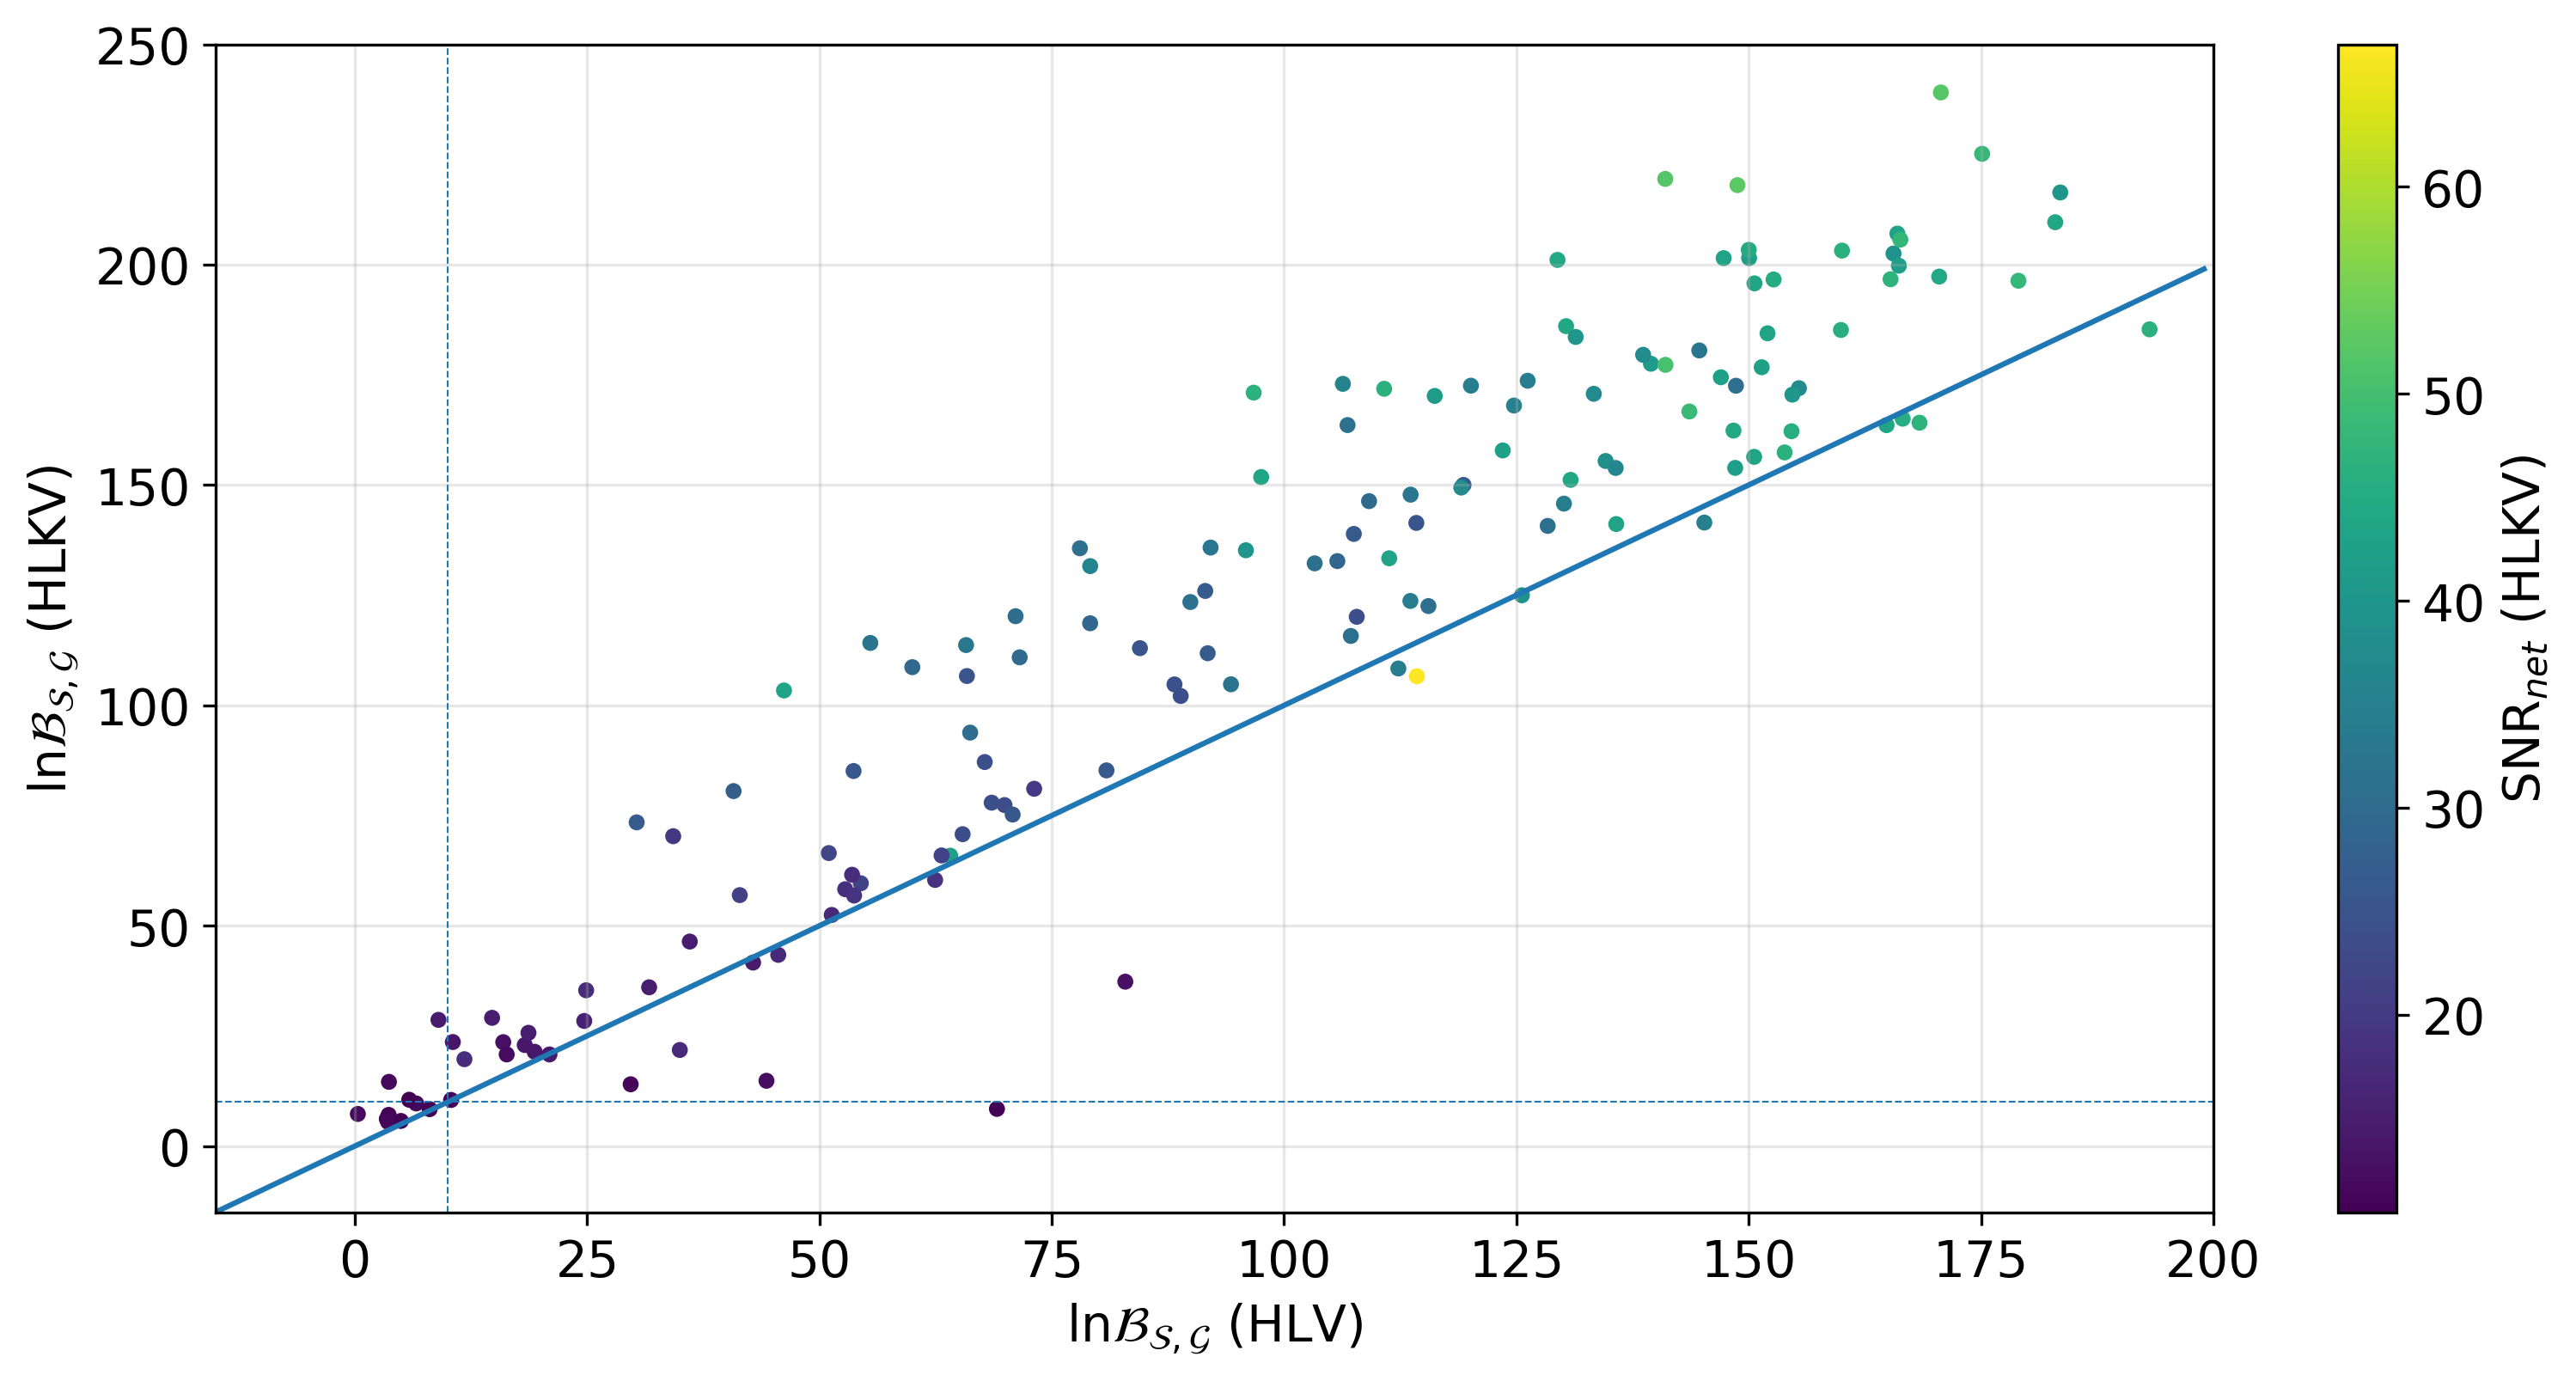}
\end{minipage}
    \caption{Left panel shows $\ln \mathcal{B}_{\mathcal{S},\mathcal{G}}$ versus SNR$_\text{net}$ of the corresponding network. The blue dots, the orange stars and green crosses indicate injections for the HL, HLV and HLKV network respectively. Right panel shows $\ln \mathcal{B}_{\mathcal{S},\mathcal{G}}$ of the HLKV network versus that of the HLV network and the colormap indicates the SNR$_\text{net}$ of the HLV network for each injection.}
    \label{fig:BSG_HLKV}
\end{figure*}

\section{HLKV Network} \label{app:HLKV}

We expand the Bayes factor analysis to a four-detector network (HLKV) with the addition of the KAGRA detector. We inject the same set of simulated BBH signals into the network and run the \textit{BayesWave} pipeline as before. The aim is to show that the scaling $ \ln \mathcal{B}_{\mathcal{S},\mathcal{G}} \sim \mathcal{O}[\mathcal{I}N\ln\text{SNR}_{\text{net}}]$ holds beyond a three-detector network. 

We show the results of this analysis in Figure \ref{fig:BSG_HLKV}. The left panel shows the logarithmic signal-to-glitch Bayes factor $\ln \mathcal{B}_{\mathcal{S},\mathcal{G}}$ of all three detector networks versus network SNR. The right panel shows the comparison of $\ln \mathcal{B}_{\mathcal{S},\mathcal{G}}$ between the HLV and HLKV networks. The blue line indicates equal $\mathcal{B}_{\mathcal{S},\mathcal{G}}$ for the HLV and HLKV network. Both plots show further improvements in $\ln \mathcal{B}_{\mathcal{S},\mathcal{G}}$ at all SNRs with addition of the KAGRA detector. However, if we compare the plot in the right panel of Figure \ref{fig:BSG_HLKV} with Figure \ref{fig:BF_HLVsnr}, we note further improvements in $\ln \mathcal{B}_{\mathcal{S},\mathcal{G}}$ with the addition of KAGRA. According to the scaling relation given in Equation \ref{eq:BFscaleapprox}, we expect a $50\%$ improvement in the Bayes factor when adding a third detector and a $33\%$ improvement when adding a forth detector, regardless of sensitivity. This is reflected in our results in Figure \ref{fig:BF_HLVsnr}. However, since KAGRA is less sensitive compared to Virgo (see Figure \ref{fig:PSD}), we observe more scatter in $\ln \mathcal{B}_{\mathcal{S},\mathcal{G}}$. 
%If all detectors were equally sensitive, we can expect to see a uniform increase in Bayes Factor with increasing number of detectors.
