# Supplementary material for: Enhancing gravitational-wave burst detection confidence in expanded detector networks with the BayesWave pipeline
Source: arXiv:2102.10816 source file (2021-02-22)
Supplement: Supplementary file 3 [file appendix5.tex]

\section{Detectors with identical PSDs} \label{app:equal_sensitivity}

\begin{figure}[t]
\centering
\includegraphics[width=.49\textwidth]{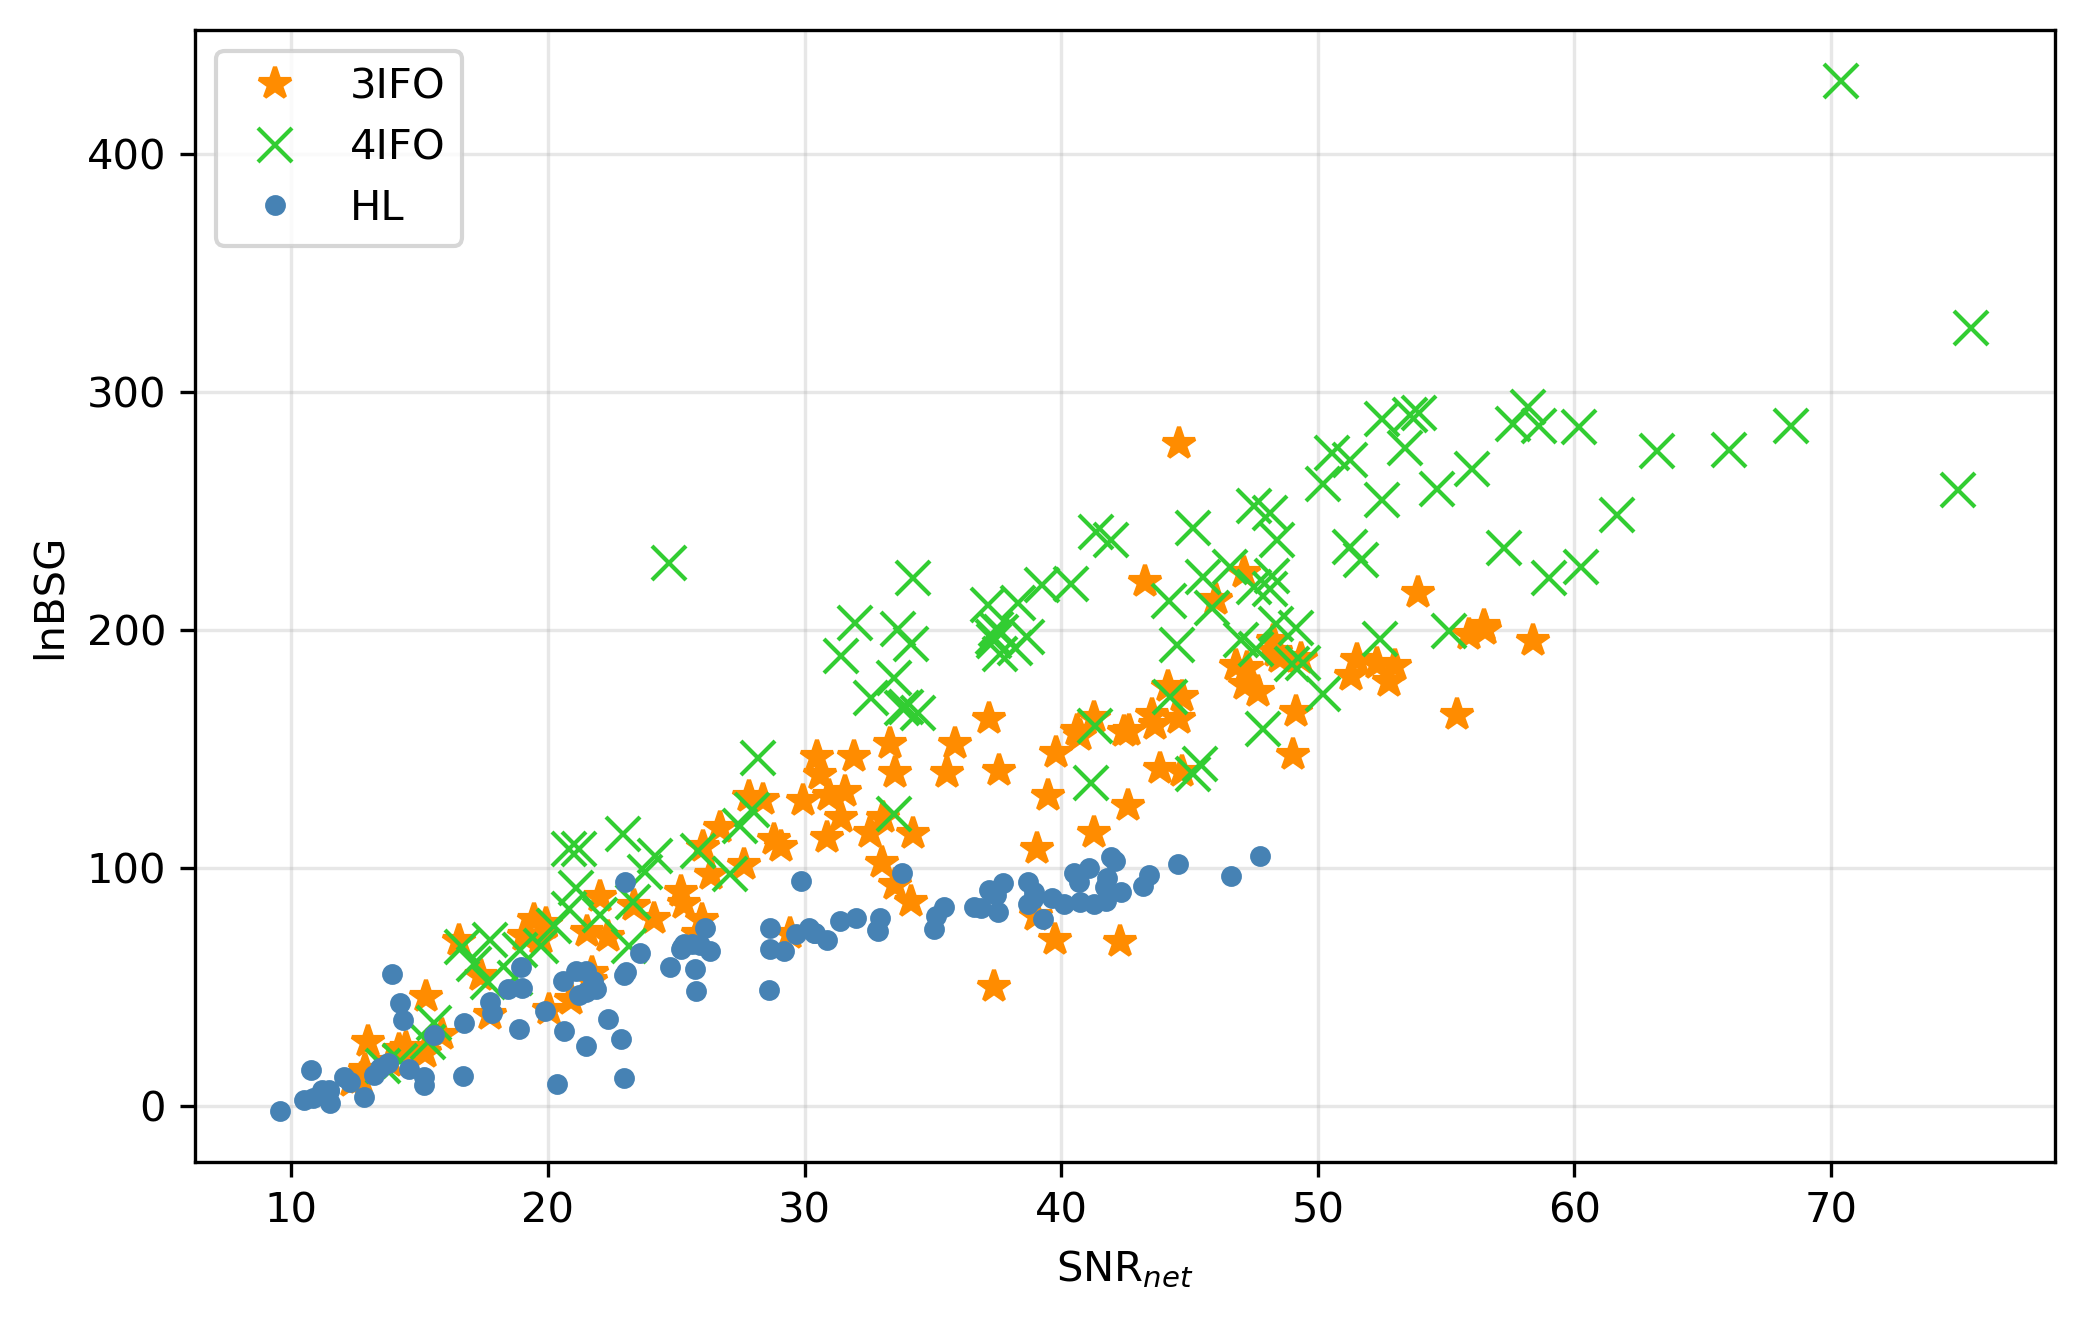}
    \caption{$\ln \mathcal{B}_{\mathcal{S},\mathcal{G}}$ of BBH injection recoveries versus network signal-to-noise ratio, SNR$_{\text{net}}$. The horizontal axis corresponds three different network SNRs: (i) for the blue dot data points it corresponds to SNR$_{\text{net}}$ of the HL network, (ii) for the orange star data points it corresponds to SNR$_{\text{net}}$ of the 3IFO network, (iii) for the green cross data points it corresponds to SNR$_{\text{net}}$ of the 4IFO network.}
    \label{fig:BSG_equal}
\end{figure}

\begin{figure*}[t]
\centering
\begin{minipage}{0.455\textwidth}
\includegraphics[width=\textwidth]{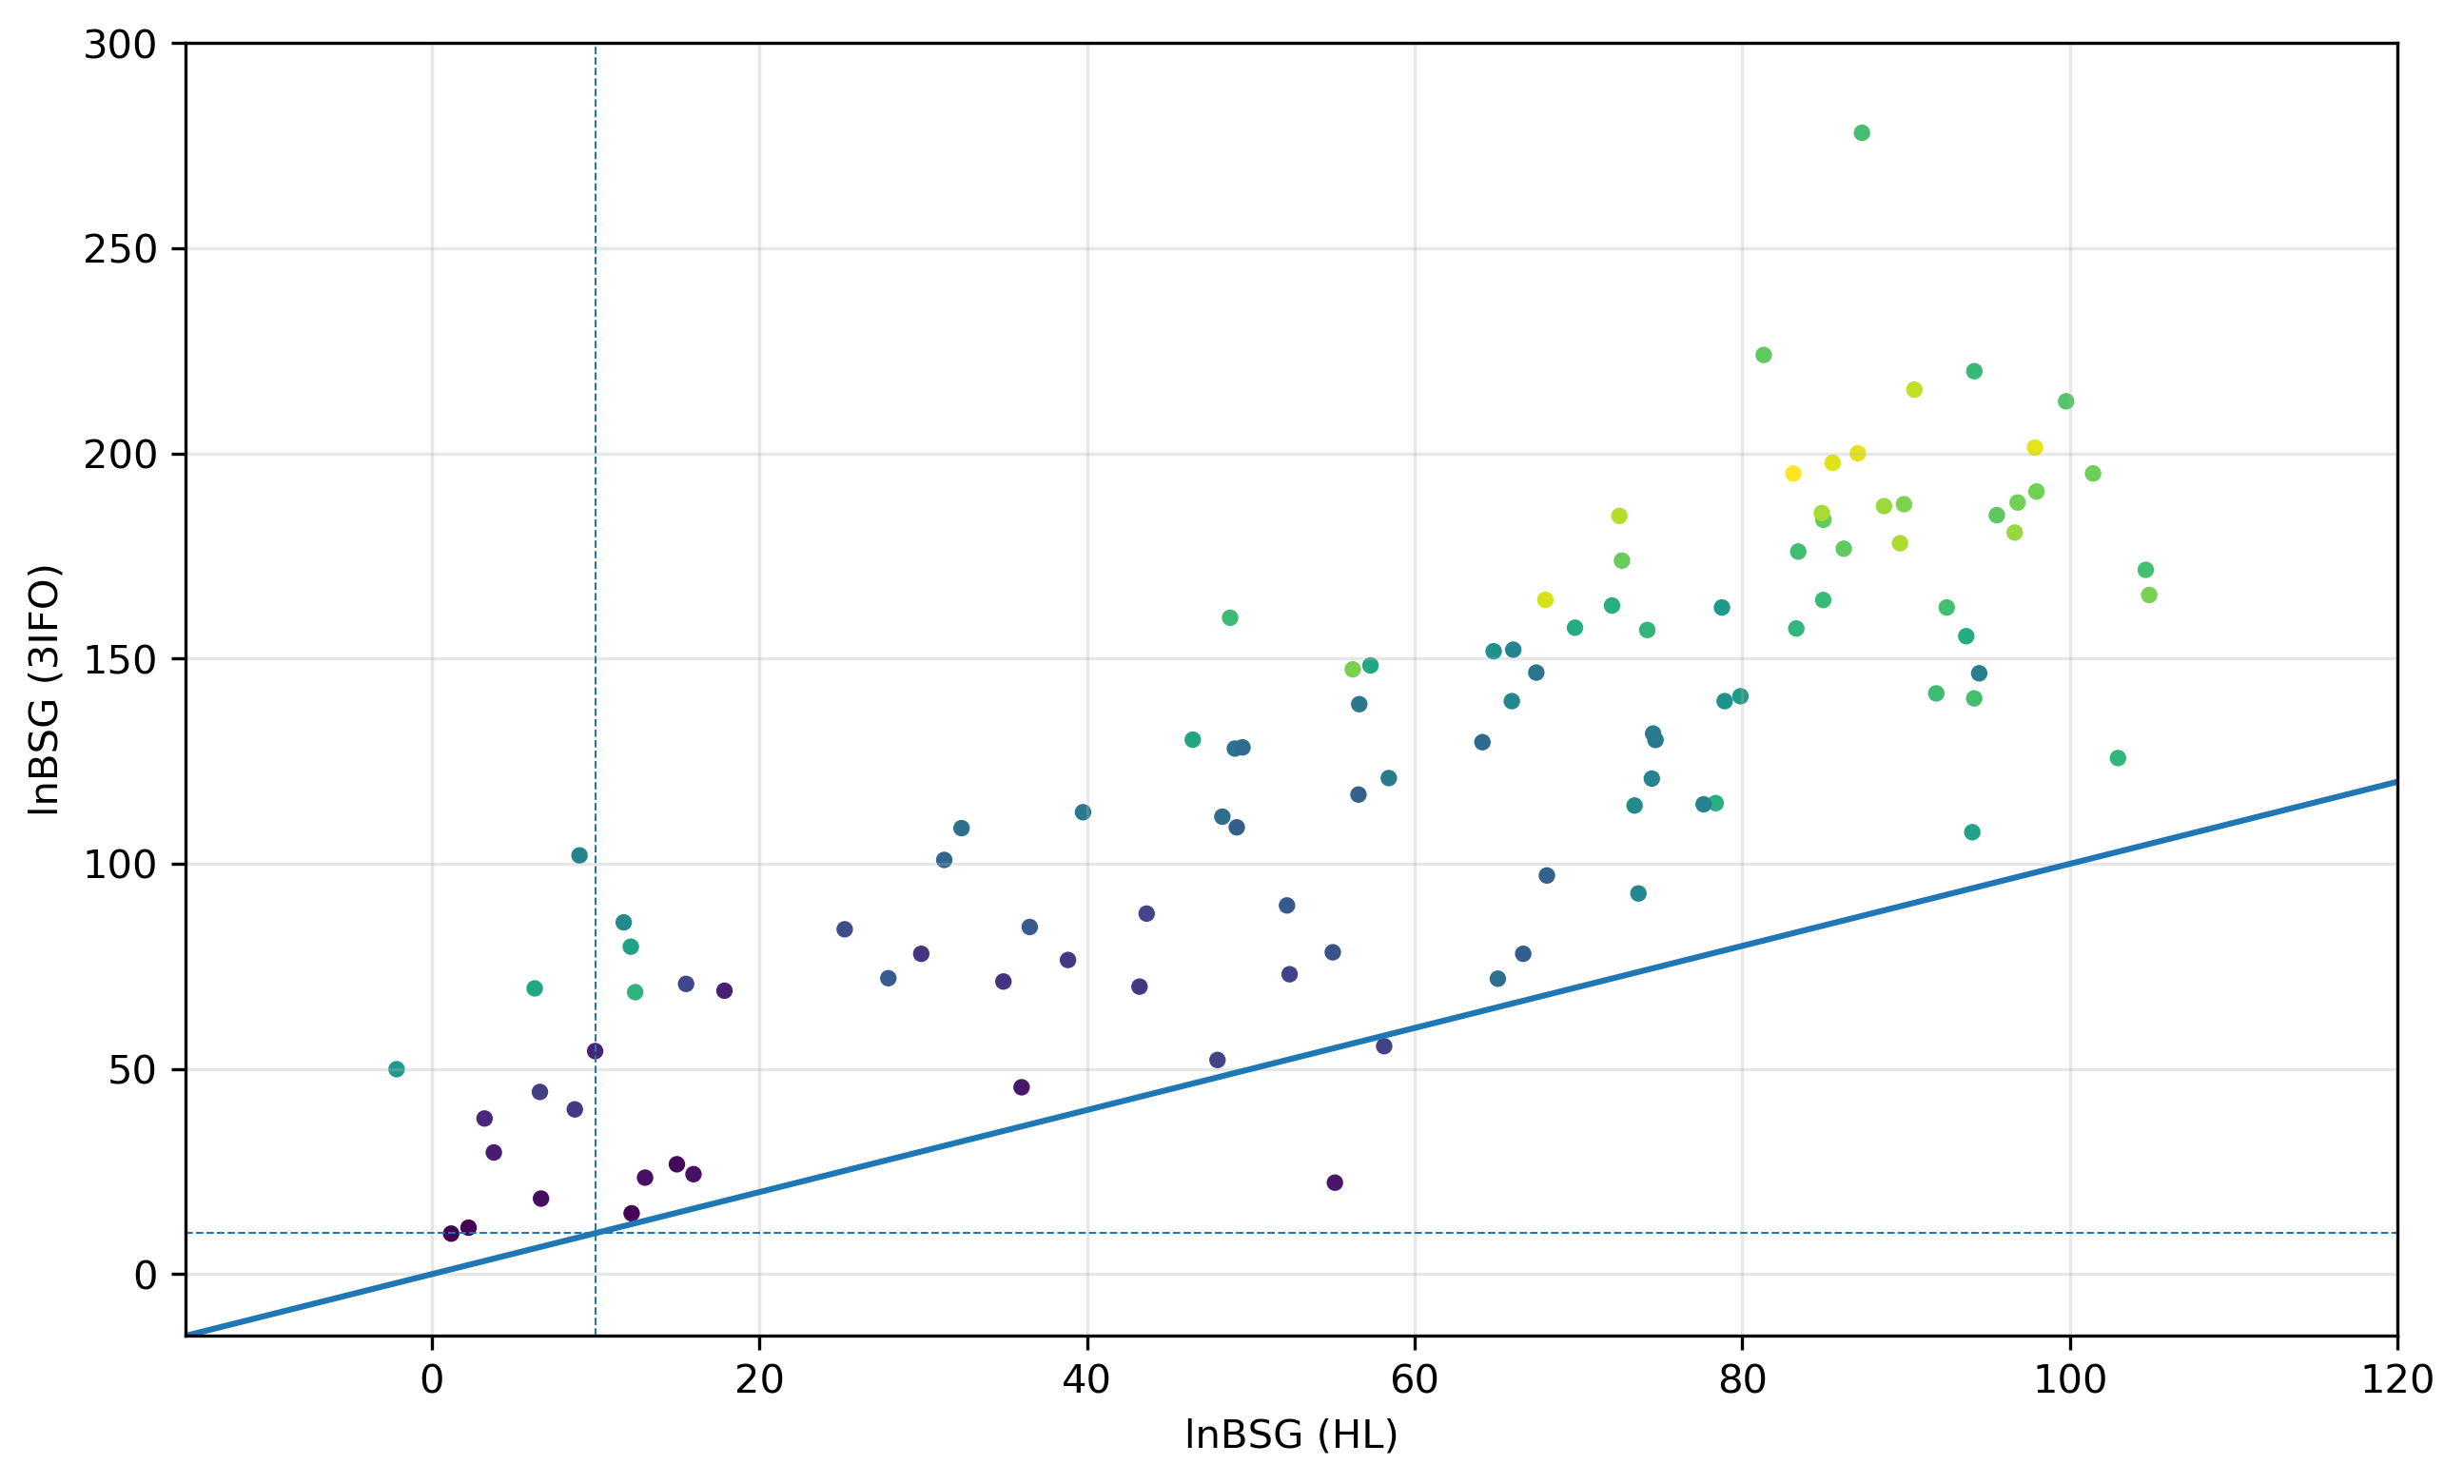}
\end{minipage}\hfill
\begin{minipage}{0.52\textwidth}
\includegraphics[width=\textwidth]{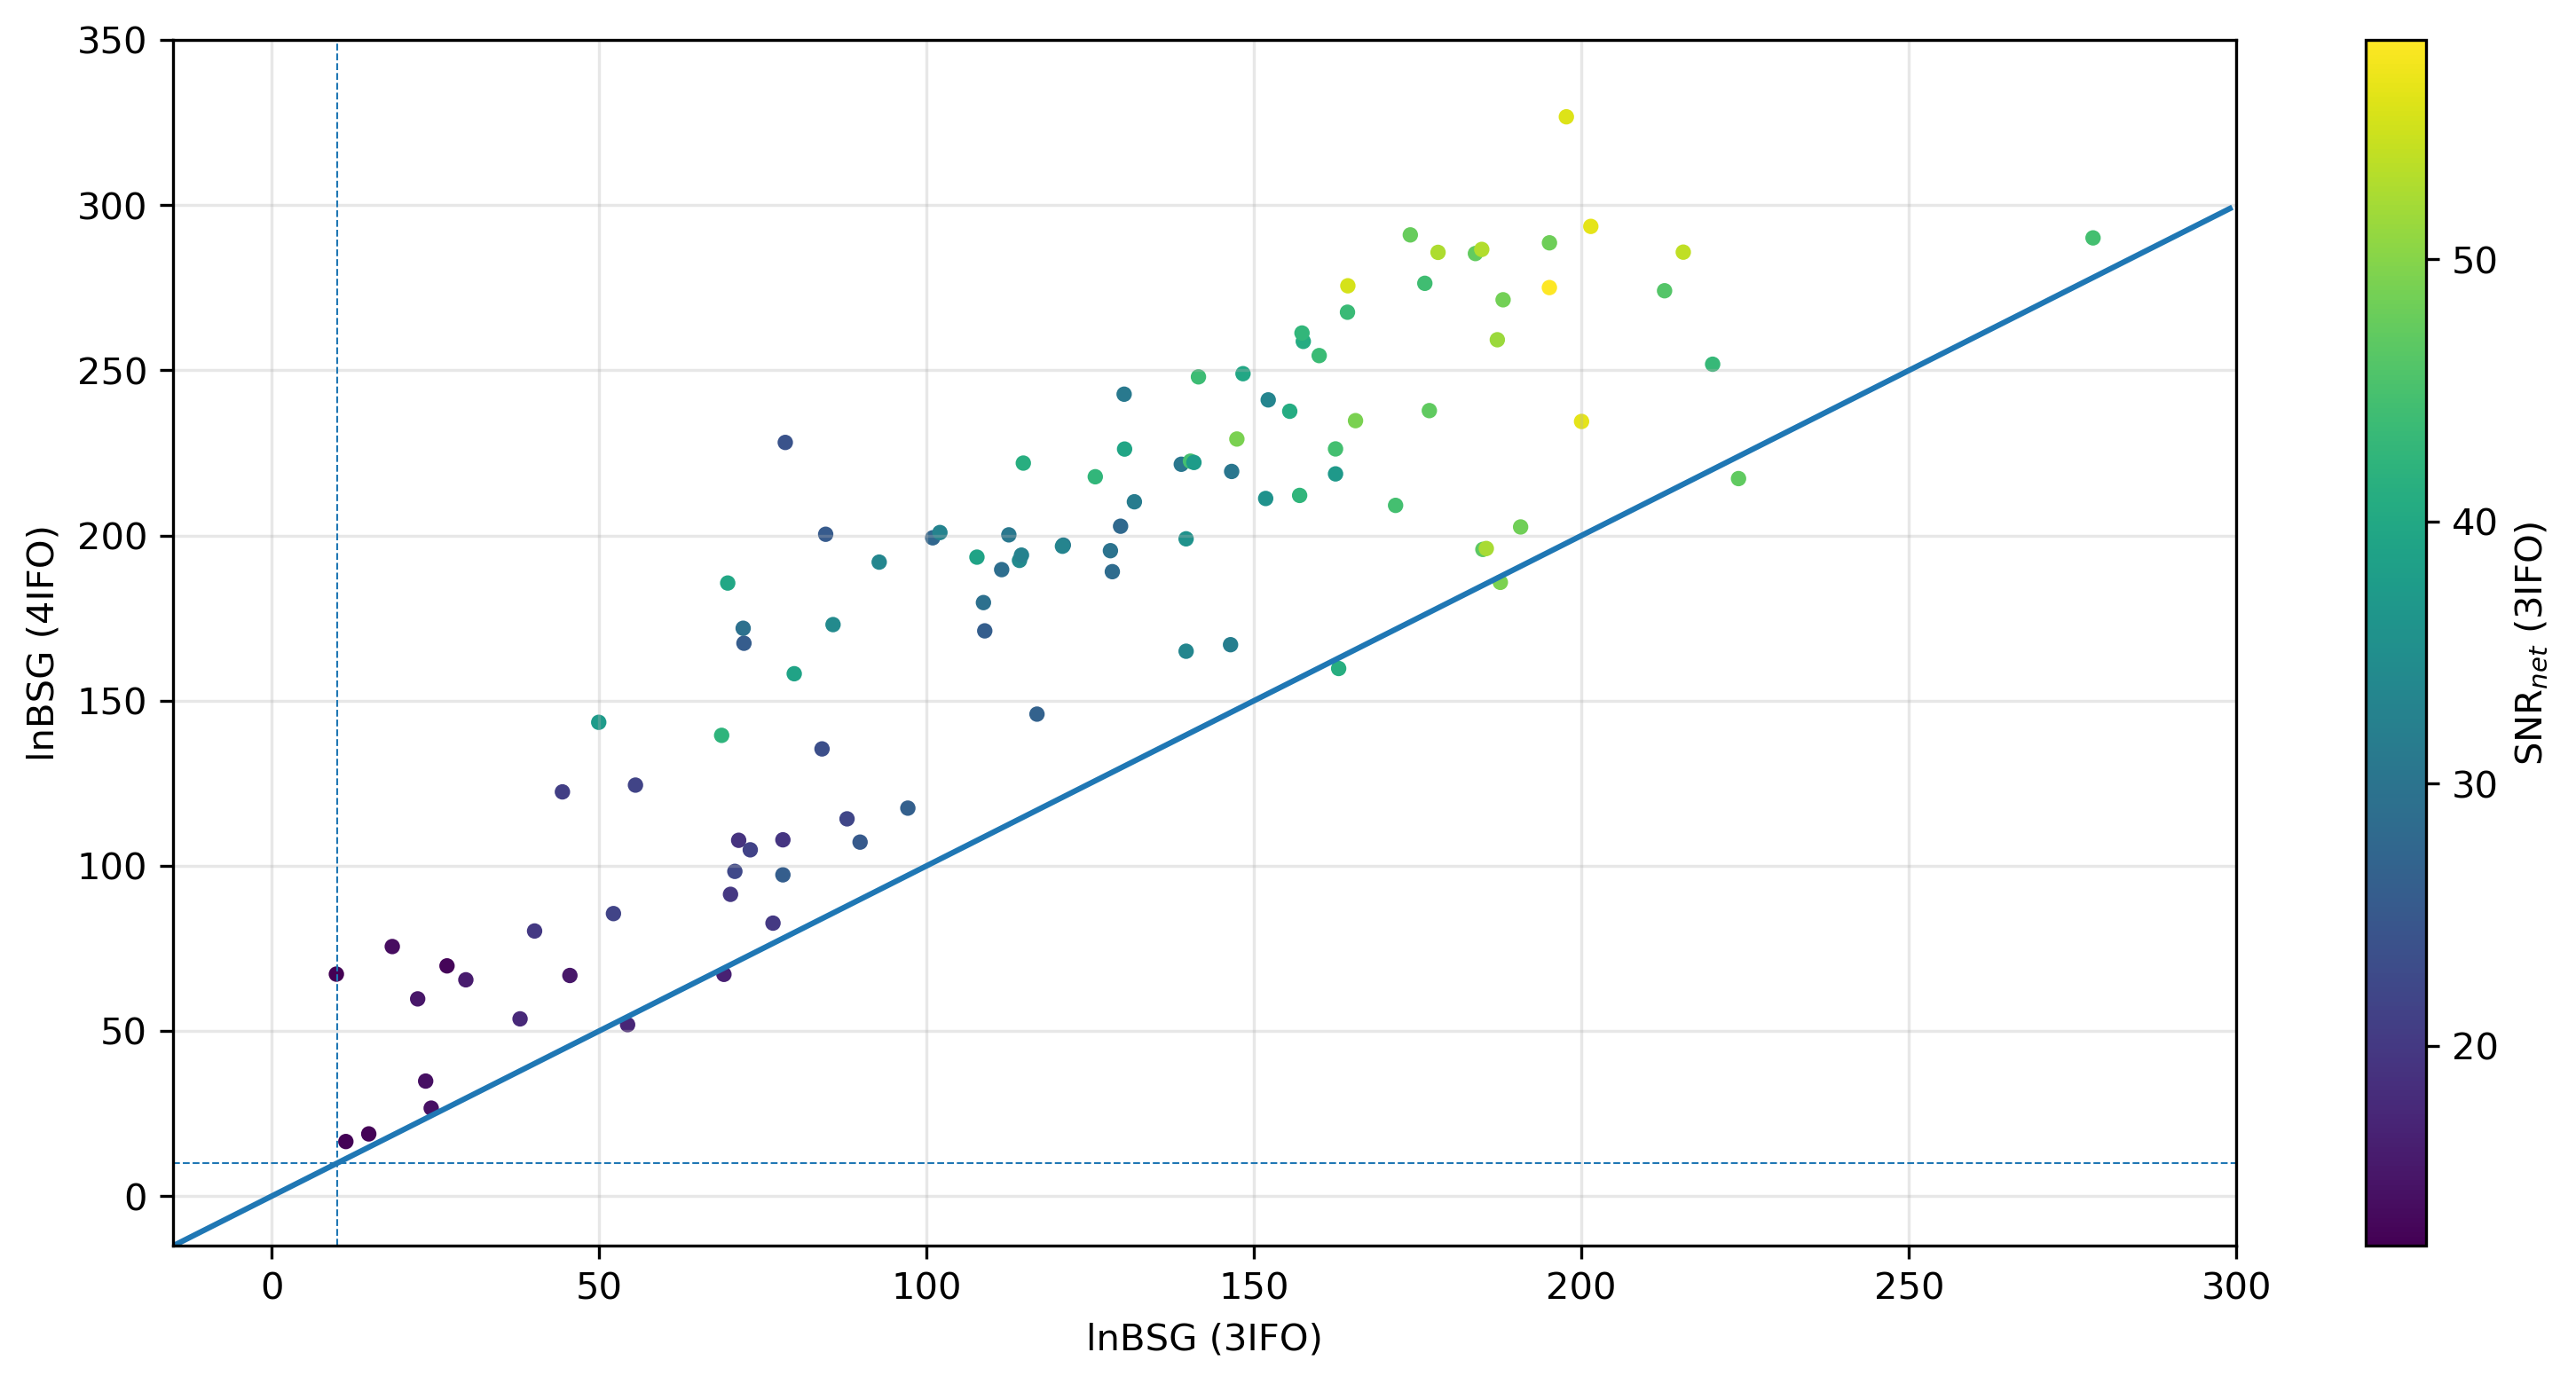}
\end{minipage}
\caption{Left panel shows $\ln \mathcal{B}_{\mathcal{S},\mathcal{G}}$ of the 3IFO network versus that of the HL network. Right panel shows $\ln \mathcal{B}_{\mathcal{S},\mathcal{G}}$ of the 4IFO network versus that of the 3IFO network. The color bar shows the SNR$_\text{net}$ of the 3IFO network for each injection and is applicable to both plots in the bottom panel. The blue lines indicate equal $\mathcal{B}_{\mathcal{S},\mathcal{G}}$ in the vertical and horizontal axes.}
    \label{fig:BSG_comparison_equal}
\end{figure*}

The predicted scaling in Equation~\ref{eq:BFscaleapprox} was derived assuming a signal has equal SNR in each detector.  However the projected sensitivities of the detectors are expected differ substantially (see Figure~\ref{fig:PSD}), which leads to different SNRs in each detector. In order to more accurately compare our analytic scaling to empirical data, we test the performance of \textit{BayesWave} with more optimal detector configurations where the detectors have same sensitivities at all frequencies. We inject the same set of BBH signals into networks of two, three and four detectors where all detectors have identical PSDs. 
%The two-detector network is simply the HL network, and the three- (3IFO) and four- (4IFO) detector networks consists of detectors identical to the Hanford and Livingston detectors, with the third and fourth detectors situated at the locations of the Virgo and KAGRA detectors respectively. 
We again use the HL, HLK, and HLKV networks, but use the projected O4 sensitivity for LIGO for all detectors.
Figure \ref{fig:BSG_equal} shows $\ln \mathcal{B}_{\mathcal{S},\mathcal{G}}$ as a function of SNR$_{\text{net}}$ for the HL, 3IFO and 4IFO networks. The trends are similar to those observed in the top left panel of Figure \ref{fig:BSG}, except that $\ln \mathcal{B}_{\mathcal{S},\mathcal{G}}$ increases more significantly with increasing number of detectors. \ysl{In Figure \ref{fig:BSG_equal}, the highest $\ln \mathcal{B}_{\mathcal{S},\mathcal{G}}$ recovered from the 3IFO and 4IFO networks are 278 and 430 respectively. This is higher compared to the highest $\ln \mathcal{B}_{\mathcal{S},\mathcal{G}}$ recovered from the HLV and HLKV networks valued at 193 and 239 respectively.}

Since the BBH waveform injections for all three detector networks are identical, we can compare the Bayes factor of the same waveform recovered from detector networks of different sizes by plotting $\ln \mathcal{B}_{\mathcal{S},\mathcal{G}}$ of two detector configurations against each other. In the left panel of Figure \ref{fig:BSG_comparison_equal} we show the plot for $\ln \mathcal{B}_{\mathcal{S},\mathcal{G}}$ of the 3IFO network versus the HL network. The best-fit least square, linear regression line has a slope of 1.55, implying a $55\%$ improvement in Bayes factor on average upon addition of a third detector. This is significantly higher than the $29\%$ improvement observed with the HLV network and closer to the analytically predicted improvement of $50\%$. In the right panel we show the plot for $\ln \mathcal{B}_{\mathcal{S},\mathcal{G}}$ the 4IFO network versus the 3IFO network which has a slope of 1.16, implying a $16\%$ improvement in Bayes factor upon increasing the detector count from three to four detectors. We compare this with the $13\%$ improvement with the HLKV network and the analytically predicted improvement of $33\%$. 

The mismatch between the empirical and predicted improvements in Bayes factor can be explained by the fact that even with identical PSDs, the SNR of a signal will still not be identical in all detectors. This is because the  
%different detectors locations on earth. The predicted improvements assume detectors with identical PSDs at the same location, where all detectors accorss the network receive GW signal at equal SNRs. For our analysis, 
detectors are geographically separated and hence they have different antenna patterns which results in each detector receiving the same signal at different SNRs despite having identical PSDs. 
%In particular, we note that the location KAGRA 
%Also notice that the predicted improvement in Bayes factor largely differs from the empirical improvement with increasing $\mathcal{I}$. This is due to the increased variance in SNR of the signal received across larger detector network which suppresses the increase Bayes factor. 
%Hence, they are not equally sensitive to all parts of the sky and as a result each detector still detects the same signal at different SNRs even though the PSDs are the same.  
%
